# Supplementary material for: PhD Thesis. Computer-Aided Assessment of Tuberculosis with Radiological Imaging: From rule-based methods to Deep Learning
Source: arXiv:2205.15909 source file (2022-05-31)
Supplement: Supplementary file 3 [file SOTA_table.tex]

\chapter{SOTA Complete table}\label{ap:SOTA}
Just include the table which originates \ref{ch1:fig:SOTA1} if is completed on time
